# Supplementary material for: Electronic control and switching of entangled spin state using anisotropy and exchange in the three-particle paradigm
Source: arXiv:2112.05223 source file (2022-07-15)
Supplement: Supplementary file 1 [file Supplementary_Data.pdf]

# Electronic control and switching of entangled spin state using anisotropy and exchange in the three-particle paradigm
## Supplementary Information

### 1. Origin of Hopping Term From a Transformation of the Two Impurity Anderson Model

In this supplementary, we derive the origin of the hopping term used in the paper, and in the process show a derivation of our total Hamiltonian. We first begin with a review of the two impurity Anderson model (TIAM), which is an extension of the the single impurity Anderson model [1]. The Hamiltonian of the TIAM model is,

$$\mathcal{H} = \mathcal{H}_{\text{imp}} + \mathcal{H}_{\text{band}} + V_{\text{band-imp}}, \tag{1}$$

where, for simplicity, the impurity has only two accessible levels (one for each spin). The first term is the impurity energy term,

$$\mathcal{H}_{\text{imp}} = \sum_{i\sigma} \epsilon_i \hat{n}_{d_{i\sigma}} + U_i \hat{n}_{d_{i\uparrow}} \hat{n}_{d_{i\downarrow}}, \tag{2}$$

where $\epsilon_i$ is the energy of impurity $i \in \{2, 3\}$, $U_i$ is the Coulombic repulsion of that impurity, $\hat{n}_{d_{i\sigma}} = \hat{d}^{\dagger}_{i\sigma}\hat{d}_{i\sigma}$ is the number operator of impurity $i$ with state $\sigma$, and $\hat{d}^{\dagger}_{i\sigma}/\hat{d}_{i\sigma}$ the second-quantization creation/annihilation operators of that state, respectively. The second term describes the electrons in a metal

$$\mathcal{H}_{\text{band}} = \sum_{\mathbf{k}\sigma} \epsilon_{\mathbf{k}} \hat{c}^{\dagger}_{\mathbf{k}\sigma}\hat{c}_{\mathbf{k}\sigma}, \tag{3}$$

where $\epsilon_{\mathbf{k}}$ is the energy of the band $\mathbf{k}$, and $\hat{c}^{\dagger}_{\mathbf{k}\sigma}/\hat{c}_{\mathbf{k}\sigma}$ create/annihilate an electron with wave number $\mathbf{k}$ and spin $\sigma$ in that band, respectively. The last term describes the coupling of the bands to the impurities,

$$V_{\text{band-imp}} = \sum_{i\mathbf{k}\sigma} t_{i\mathbf{k}} \hat{c}^{\dagger}_{\mathbf{k}\sigma}\hat{d}_{i\sigma} + h.c., \tag{4}$$

where $t_{i\mathbf{k}}$ is the coupling constant. When one applies a generalized form of the Schrieffer-Wolff transformation [2] to the TIAM model, one obtains a transformed Hamiltonian $\mathcal{H}'$ that can be separated into six terms,

$$\mathcal{H}' = \mathcal{H}_0 + \mathcal{H}'_0 + \mathcal{H}_{\text{dir}} + \mathcal{H}_{\text{exch}} + \mathcal{H}_{\text{pair-tunnel}} + \mathcal{H}_{\text{imp-imp}}. \tag{5}$$

The first two terms are diagonal in the spin space of the impurities,

$$\mathcal{H}_0 = \mathcal{H}_{\text{imp}} + \mathcal{H}_{\text{band}}, \tag{6}$$

and,

$$\mathcal{H}_0' \equiv -\sum_{i\mathbf{k}\sigma} \left( W^{ii}_{\mathbf{kk}} + \frac{1}{2} J^{ii}_{\mathbf{kk}} \hat{n}_{\hat{d}_{i-\sigma}} \right) \hat{n}_{\hat{d}_{i\sigma}}, \tag{7}$$

where the coupling constants are defined as,

$$W^{i'i}_{\mathbf{k}'\mathbf{k}} \equiv \frac{1}{2} t_{i'\mathbf{k}'} t^*_{i\mathbf{k}} \left( \frac{1}{\epsilon_{\mathbf{k}'} - \epsilon_{i'}} + \frac{1}{\epsilon_{\mathbf{k}} - \epsilon_i} \right), \tag{8}$$

$$J^{i'i}_{\mathbf{k}'\mathbf{k}} \equiv t_{i'\mathbf{k}'} t^*_{i\mathbf{k}} \left( \frac{1}{\epsilon_{\mathbf{k}'} - \epsilon_{i'} - U_{i'}} + \frac{1}{\epsilon_{\mathbf{k}} - \epsilon_i - U_i} - \frac{1}{\epsilon_{\mathbf{k}'} - \epsilon_{i'}} - \frac{1}{\epsilon_{\mathbf{k}} - \epsilon_i} \right). \tag{9}$$

The third term is is the direct (spin-independent) interaction,

$$\mathcal{H}_{\text{dir}} \equiv \sum_{i\mathbf{k}\mathbf{k}'} \left( W^{ii}_{\mathbf{k}'\mathbf{k}} + \frac{1}{4} J^{ii}_{\mathbf{k}'\mathbf{k}} \left( \hat{\Psi}^\dagger_i \hat{\Psi}_i \right) \right) \left( \hat{\Psi}^\dagger_{\mathbf{k}'} \hat{\Psi}_{\mathbf{k}} \right), \tag{10}$$

where the following generalized creation/annihilation operators have been defined,

$$\hat{\Psi}_{\mathbf{k}} \equiv \begin{pmatrix} \hat{c}_{\mathbf{k}\uparrow} \\ \hat{c}_{\mathbf{k}\downarrow} \end{pmatrix}, \tag{11}$$

$$\hat{\Psi}_i \equiv \begin{pmatrix} \hat{d}_{i\uparrow} \\ \hat{d}_{i\downarrow} \end{pmatrix}. \tag{12}$$

The fourth term is the Kondo exchange interaction

$$\mathcal{H}_{\text{exch}} \equiv -\sum_{i\mathbf{k}\mathbf{k}'} J^{ii}_{\mathbf{k}'\mathbf{k}} \left( \hat{\Psi}^\dagger_{\mathbf{k}'} \frac{\hat{\boldsymbol{\sigma}}}{2} \hat{\Psi}_{\mathbf{k}} \cdot \hat{\Psi}^\dagger_i \frac{\hat{\boldsymbol{\sigma}}}{2} \hat{\Psi}_i \right) = -\sum_{i\mathbf{k}\mathbf{k}'} J^{ii}_{\mathbf{k}'\mathbf{k}} \left( \hat{\Psi}^\dagger_{\mathbf{k}'} \hat{\mathbf{S}} \hat{\Psi}_{\mathbf{k}} \cdot \hat{\Psi}^\dagger_i \hat{\mathbf{S}} \hat{\Psi}_i \right). \tag{13}$$

The fifth term is the pair-tunneling interaction where two electrons or two holes are created at once.

$$\mathcal{H}_{\text{pair-tunnel}} \equiv \frac{1}{4} \sum_{i\mathbf{k}\mathbf{k}'\sigma} J^{ii}_{\mathbf{k}'\mathbf{k}} \hat{c}^\dagger_{\mathbf{k}-\sigma} \hat{c}^\dagger_{\mathbf{k}'\sigma} \hat{d}_{i\sigma} \hat{d}_{i-\sigma} + h.c. \tag{14}$$

The last term does not appear when one transforms the single-impurity Anderson model,

$$\mathcal{H}_{\text{imp-imp}} \equiv -\frac{1}{2} \sum_{i \neq j} \sum_{\mathbf{k}\sigma} \left( W^{ij}_{\mathbf{kk}} + \frac{1}{2} \tilde{J}^{ij}_{\sigma} \right) \hat{d}^\dagger_{i\sigma} \hat{d}_{j\sigma} + h.c., \tag{15}$$

where,

$$\tilde{J}^{i'i}_{\sigma} \equiv t_{i'\mathbf{k}} t^*_{i\mathbf{k}} \left( \frac{\hat{n}_{\hat{d}_{i'-\sigma}}}{\epsilon_{\mathbf{k}} - \epsilon_{i'} - U_{i'}} + \frac{\hat{n}_{\hat{d}_{i-\sigma}}}{\epsilon_{\mathbf{k}} - \epsilon_i - U_i} - \frac{\hat{n}_{\hat{d}_{i'-\sigma}}}{\epsilon_{\mathbf{k}} - \epsilon_{i'}} - \frac{\hat{n}_{\hat{d}_{i-\sigma}}}{\epsilon_{\mathbf{k}} - \epsilon_i} \right). \tag{16}$$

This term represents a second-order hopping between sites mediated by the conduction electron levels. In other words, it represents an electron hopping away from one impurity into the conduction band, followed by an electron hopping from the conduction band to the second impurity. The first two terms of the transformed Hamiltonian adjust the energy level of the system, and can be incorporated to redefine the energy levels. The third term can be absorbed into the bands, and the fifth term can be neglected because it is energetically unfavorable in this second-order treatment. There are two surviving terms, namely the Kondo exchange interaction and impurity-impurity interaction terms, that describe the transformed TIAM model, which we call the two-site Kondo model,

$$\mathcal{H}_{2K} \equiv \mathcal{H}_{\text{exch}} + \mathcal{H}_{\text{imp-imp}}. \tag{17}$$

This model can be generalized to larger spin for the impurities. First, a simple notation change is made,

$$\hat{\Psi}^{\dagger}_{\mathbf{k}'}\hat{\mathbf{S}}\hat{\Psi}_{\mathbf{k}} \equiv \hat{\Psi}^{\dagger}_{\mathbf{k}'}\mathbf{S_1}\hat{\Psi}_{\mathbf{k}}, \tag{18}$$

and then the spin sum over $\sigma$ is expanded to a sum over all $\mu$ spin degrees of freedom in the impurities of any spin $S$,

$$\mathcal{H}_{2K} = -\sum_{i,\mathbf{k},\mathbf{k}'} J^{ii}_{\mathbf{k}'\mathbf{k}} \left(\hat{\Psi}^{\dagger}_{\mathbf{k}'}\mathbf{S_1}\hat{\Psi}_{\mathbf{k}} \cdot \hat{\Psi}^{\dagger}_{i}\hat{\mathbf{S}}_i\hat{\Psi}_i\right) - \frac{1}{2}\sum_{i\neq j}\sum_{\mathbf{k},\mu}\left(W^{ij}_{\mathbf{kk}} + \frac{1}{2}\tilde{J}^{ij}_{\mu}\right)\hat{d}^{\dagger}_{i\mu}\hat{d}_{j\mu} + h.c. \tag{19}$$

In order to isolate the spin space of this model, the momentum index $\mathbf{k}$ is dropped,

$$\mathcal{H}_{2K} = -\sum_{\mu,\mu',i} J^{ii}\hat{\mathbf{S}}_i \cdot \hat{d}^{\dagger}_{\mu,i}\hat{\boldsymbol{\sigma}}_{\mu,\mu'}\hat{d}_{\mu',i} - \frac{1}{2}\sum_{i\neq j}\sum_{\mu}\left(W^{ij} + \frac{1}{2}\tilde{J}^{ij}_{\mu}\right)\hat{d}^{\dagger}_{i\mu}\hat{d}_{j\mu} + h.c. \tag{20}$$

The constants can then be redefined, e.g., $J_{Ki} \equiv -2J^{ii}$ and $t_{\mu,ij} = -1/2(W^{ij} + \tilde{J}^{ij}_{\mu}/2)$, so that,

$$\mathcal{H}_{\text{three-spin}} = \frac{1}{2}\sum_{\mu,\mu',i} J_{Ki}\hat{\mathbf{S}}_i \cdot \hat{d}^{\dagger}_{\mu,i}\hat{\boldsymbol{\sigma}}_{\mu,\mu'}\hat{d}_{\mu',i} + \sum_{\mu} t_{\mu,23}\hat{d}^{\dagger}_{\mu,2}\hat{d}_{\mu,3} + h.c. \tag{21}$$

Finally one can see that the problem in spin space is now constructed of interactions between three spin operators: $\hat{\mathbf{S}}_1$, $\hat{\mathbf{S}}_2$, and $\hat{\mathbf{S}}_3$, and a hopping term. Assuming that the hopping term is independent of the spin of the impurities, $t_{23\mu} = t \ \forall \ \mu$, one finds,

$$\mathcal{H}_{\text{three-spin}} = \mathcal{H}_{\text{K}} + \mathcal{H}_{\text{t}}, \tag{22}$$

where,

$$\mathcal{H}_{\text{K}} = \frac{1}{2}\sum_{\mu,\mu',i=2,3} J_{\text{K}i}\hat{\mathbf{S}}_i \cdot \hat{d}^{\dagger}_{\mu,i}\hat{\boldsymbol{\sigma}}_{\mu,\mu'}\hat{d}_{\mu',i}, \tag{23}$$

and,

$$\mathcal{H}_{\text{t}} = \sum_{\mu}\left\{t\hat{d}^{\dagger}_{\mu,2}\hat{d}_{\mu,3} + h.c.\right\}. \tag{24}$$

Spin interactions between the impurities and other dynamics can be included, like magnetic anisotropy, to obtain the total Hamiltonian used in the paper,

$$\mathcal{H} = \mathcal{H}_{\mathrm{H}} + \mathcal{H}_{\mathrm{K}} + \mathcal{H}_{\mathrm{A}} + \mathcal{H}_{\mathrm{t}}. \tag{25}$$

[1] Anderson P W 1966 *Physical Review Letters* **17** 95–97 URL https://link.aps.org/doi/10.1103/PhysRevLett.17.95

[2] Schrieffer J R and Wolff P A 1966 *Physical Review* **149** 491–492 URL https://link.aps.org/doi/10.1103/PhysRev.149.491
